# Supplementary material for: Numerical analysis of three-dimensional magnetohydrodynamic effects in an inductively coupled plasma wind tunnel
Source: arXiv:2504.07218 source file (2026-08-03)
Supplement: Supplementary file 1 [file appendix.tex]

\section*{Appendix}
\appendix
    \begin{appendices} 
    
    \end{appendices}
